# Supplementary material for: Fully Sparse Fusion for 3D Object Detection
Source: arXiv:2304.12310 source file (2024-04-28)
Supplement: Supplementary file 1 [file appendix_decoder_layers.tex]

\begin{table}[!h]
\begin{center}
\resizebox{0.5\columnwidth}{!}{%
\begin{tabular}{@{}c|cc@{}}
\toprule
$\#$Refined Layers & mAP  & NDS  \\ \midrule
0                 & 68.0    &71.3     \\  
1                 & 70.4    &72.7 \\
2                 & 70.4    &72.8     \\ \bottomrule
\end{tabular}
}
\end{center}
\caption{Result of the different number of query refinement layers. 0 means directly merging the LiDAR query boxes and camera query boxes via NMS.}
\label{tab:num_refine_layers}
\end{table}
