# Supplementary material for: Fully Sparse Fusion for 3D Object Detection
Source: arXiv:2304.12310 source file (2024-04-28)
Supplement: Supplementary file 2 [file appendix_latency.tex]

\begin{table}[h]
\begin{center}
\resizebox{1.0\columnwidth}{!}{%
\begin{tabular}{l|ccc|c}
\toprule
Method      & Image \dag      & LiDAR backbone \ddag      & Predictor \P & Overall (ms) \\ \midrule
TransFusion & 30         & 228        & 126  & 384          \\
FSF (ours)  & 52         & 54         & 35   & 141          \\ \bottomrule
\end{tabular}%
}
\end{center}
\caption{
Latency comparison on Argoverse 2, which covers a $400m \times 400m$ area. The details of \dag, \ddag, \P ~are in text.
}
\label{tab:detailed_latency}
\end{table}
