# Supplementary material for: Fully Sparse Fusion for 3D Object Detection
Source: arXiv:2304.12310 source file (2024-04-28)
Supplement: Supplementary file 3 [file appendix_recalls.tex]

\begin{table*}[!ht]
\begin{center}
\resizebox{0.8\textwidth}{!}{
\begin{tabular}{l|c|cccccccccc}
\toprule
Methods  & mAR  & Car  & Truck & Bus  & Trailer & C.V. & Pedestrian & Motor. & Bicycle & T.C. & Barrier \\ \midrule
FSD            & 67.3 & 82.0 & 65.8 & 66.9 & 31.7  & 25.1 & 90.8 & 75.1 & 75.0 & 83.6 & 77.2       \\
FSD + Painting & 69.0 & 82.7 & 67.3 & 66.9 & 33.4  & 28.0 & 92.2 & 77.6 & 79.1 & 84.4 & 78.3       \\
\name          & 71.7 & 83.1 & 68.2 & 68.9 & \textbf{37.3} & 29.1 & 93.0 & 78.8 & \textbf{84.3} & \textbf{92.3} & \textbf{82.0}   \\
\midrule
Improvement$^*$ & +4.4 & +1.1 & +2.4 & +2.0 & +5.6 & +4.0 & +2.2 & +3.7 & +9.3 & +8.7 & +4.8 \\
\bottomrule
\end{tabular}%
}
\end{center}
\caption{
Comparison on \emph{recall} where the distance threshold is $0.5m$.
mAR: mean average recall.
$^*$: The FSF's improvement over FSD.
C.V.: Construction Vehicle. 
Motor.: Motorcycle.
T.C: Traffic Cone. 
We mark some items with significant improvement over ``FSD + Painting'' in \textbf{bold}.
}
\label{tab:appendix_recalls}
\end{table*}
